# Supplementary material for: Transferable Learning of Reaction Pathways from Geometric Priors
Source: arXiv:2504.15370 ancillary file (2025-04-21)
Supplement: Supplementary file 1 [file SI.pdf]

# Supporting Information: Transferable Learning of Reaction Pathways from Geometric Priors

Juno Nam,[†,‡] Miguel Steiner,[†] Max Misterka,[¶] Soojung Yang,[§] Avni Singhal,[†] and Rafael Gómez-Bombarelli[*,†]

†*Department of Materials Science and Engineering, Massachusetts Institute of Technology, Cambridge, Massachusetts 02139, United States*

‡*Energy Storage Research Alliance, Argonne National Laboratory, 9700 South Cass Avenue, Lemont, Illinois 60439, United States*

¶*Department of Mathematics, Massachusetts Institute of Technology, Cambridge, Massachusetts 02139, United States*

§*Computational and Systems Biology Program, Massachusetts Institute of Technology, Cambridge, Massachusetts 02139, United States*

E-mail: rafagb@mit.edu

# Contents

**S1 Model and Training** **S-3**

S1.1 Model Architecture . . . . . . . . . . S-3

S1.2 Spline Interpolation for MEPIN-**G** . . . . . . . . . . S-3

S1.3 Training Details and Algorithms . . . . . . . . . . S-4

S1.4 Hyperparameters . . . . . . . . . . S-5

**S2 Dataset** **S-8**

S2.1 Dataset Preparation . . . . . . . . . . S-8

S2.2 Comparison with the Original Dataset . . . . . . . . . . S-8

**S3 Additional Results** **S-10**

S3.1 Saddle-Point Optimization . . . . . . . . . . S-10

S3.2 Inference Example: Energy vs. Geometry . . . . . . . . . . S-11

S3.3 Computational Cost . . . . . . . . . . S-12

**References** **S-13**

# S1 Model and Training

## S1.1 Model Architecture

We modified the PaiNN[S1] architecture to parametrize the scaled difference between the reaction path and the initial interpolation, denoted as $\phi(x_{\mathrm{R}}, x_{\mathrm{P}}, a, t; \theta)$ in the main text. The message passing scheme incorporates three sets of edge information from the reactant geometry $x_{\mathrm{R}}$, product geometry $x_{\mathrm{P}}$, and interpolated geometry $x_{\mathrm{interp}}$. While $x_{\mathrm{interp}}$ is implicit in the main text, being determined by the interpolation scheme and $x_{\mathrm{R}}$, $x_{\mathrm{P}}$, and $t$, we make it explicit here in the model argument: $\phi(x_{\mathrm{R}}, x_{\mathrm{P}}, x_{\mathrm{interp}}, a, t; \theta)$. Edges are constructed between atom pairs with distances less than $r_{\mathrm{cut}} = 6$ Å in either $x_{\mathrm{R}}$ or $x_{\mathrm{P}}$. Note that the edge construction is independent of $x_{\mathrm{interp}}$, allowing edges to be computed once per reaction for all images in a batch, which improves training efficiency. To handle atom pairs with small distances in $x_{\mathrm{interp}}$ due to linear interpolation, we shift all the distances by $r_{\mathrm{shift}} = 0.5$ Å when computing radial basis function outputs.

Similarly to our previous work[S2], we use separate filters for each geometry and combine their outputs via elementwise addition in the continuous-filter convolution layers. Finally, to break mirror symmetry in the output, we adopt the vector products from the ChiroPaiNN model[S3]. The readout layer predicts a single SE(3)-equivariant vector for each atom, corresponding to $\phi(x_{\mathrm{R}}, x_{\mathrm{P}}, x_{\mathrm{interp}}, a, t; \theta)$.

## S1.2 Spline Interpolation for MEPIN-G

The geodesic interpolation[S4] produces a sequence of images from reactant to product by minimizing geometric length. To create a differentiable initial interpolation path for MEPIN-**G**, we use a $C^2$-continuous piecewise cubic B-spline, with geodesic images as control points. We generate $N_{\mathrm{control}} = 11$ geodesic images from $x_{\mathrm{R}}$ ($k = 1$) to $x_{\mathrm{P}}$ ($k = N_{\mathrm{control}}$), align them to the reactant, and denote them as $\{x_{\mathrm{geodesic},k}\}_{k=1}^{N_{\mathrm{control}}}$.

For global interpolation parameter $t$, the path is split into $N_{\mathrm{control}} + 1$ segments, with

segment index $i_{\text{seg}} = \lfloor (N_{\text{control}} + 1)t \rfloor$ and local interpolation parameter $t_{\text{seg}} = (N_{\text{control}} + 1)t - \lfloor (N_{\text{control}} + 1)t \rfloor \in [0, 1]$. Each cubic B-spline segment is then defined as[S5]:

$$x_{\text{interp}}(t_{\text{seg}}) = \frac{1}{6}\left[(-t^3 + 3t^2 - 3t + 1)x_0 + (3t^3 - 6t^2 + 4)x_1 + (-3t^3 + 3t^2 + 3t + 1)x_2 + t^3 x_3\right], \tag{S1}$$

where $(x_0, x_1, x_2, x_3)$ are the control points of the segment, defined as $x_i = x_{\text{geodesic},k_i}$ with:

$$\begin{aligned} k_0 &= \max(1, i_{\text{seg}} - 1), \\ k_1 &= \min(\max(1, i_{\text{seg}}), N_{\text{control}}), \\ k_2 &= \min(i_{\text{seg}} + 1, N_{\text{control}}), \\ k_3 &= \min(i_{\text{seg}} + 2, N_{\text{control}}). \end{aligned} \tag{S2}$$

While this parametrization ensures that $t = 0$ and $t = 1$ correspond to $x_{\text{R}}$ and $x_{\text{P}}$, respectively, the spline path does not pass exactly through the intermediate control points. This is acceptable, as the spline serves only as an initial guess, and the flexibility of the parametrized model allows it to learn the true reaction path during training.

## S1.3 Training Details and Algorithms

The training algorithm for geodesic pre-training for MEPIN-**L** is given in Algorithm S1. We applied two augmentations in line 4: (1) swapping the reactant and product, and (2) rotating $x_{\text{P}}$ relative to $x_{\text{R}}$ using a small rotation matrix with Euler angles sampled from $\mathcal{N}(0, \sigma_{\text{angle}}^2)$, with $\sigma_{\text{angle}} = 0.05$ rad. To stabilize the training, we clipped loss values exceeding 100 (disabling gradient computation) and applied gradient clipping on parameters.

The training algorithms for energy-based training of MEPIN-**L** and **G** are shown in Algorithm S2 and Algorithm S3, respectively. For MEPIN-**G**, augmentation is disabled to leverage cached geodesic control points computed from unaugmented geometries. As in geodesic pre-training, we apply clipping to both loss values and parameter gradients

(see Table S3). In practice, the potential energy (line 9) for geometry $x$ is computed as $U(x)-U(x_{\mathrm{R}})$, preserving parameter gradients through $x$ while ensuring consistent application of loss clipping and flux loss logging across different reactions. We used the dxtb package[S6] to perform batched energy evaluations at the GFN1-xTB level[S7].

For all training, UPDATE uses the Adam optimizer[S8], with a maximum of 100 epochs and early stopping based on validation loss with a patience of 20 epochs.

**Algorithm S1** Geodesic pre-training (MEPIN-**L**)

**Require:** Reactant-product dataset $\mathcal{D}$, initial parameters $\theta$
1: **repeat**
2:   **for** $r = 1, \cdots, N_{\mathrm{rxn}}$ **do** ▷ *Reaction batch*
3:     Sample reactant and product pair $(x_{\mathrm{R}}^{(r)}, x_{\mathrm{P}}^{(r)}, a) \sim \mathcal{D}$
4:     $x_{\mathrm{R}}^{(r)}, x_{\mathrm{P}}^{(r)} \leftarrow$ AUGMENT$(x_{\mathrm{R}}^{(r)}, x_{\mathrm{P}}^{(r)})$
5:     **for** $i = 1, \cdots, N_{\mathrm{image}}$ **do** ▷ *Image batch*
6:       Sample interpolation parameter $t_i \sim \mathcal{U}(0, 1)$
7:       $x_{\mathrm{interp},i}^{(r)} \leftarrow (1 - t_i)x_{\mathrm{R}}^{(r)} + t_i x_{\mathrm{P}}^{(r)}$ ▷ *Initial interpolant (linear)*
8:       $x_i^{(r)} \leftarrow x_{\mathrm{interp},i}^{(r)} + t_i(1 - t_i)\phi(x_{\mathrm{R}}^{(r)}, x_{\mathrm{P}}^{(r)}, x_{\mathrm{interp},i}^{(r)}, a^{(r)}, t_i; \theta)$ ▷ *Predicted path image*
9:       $\dot{q}_i^{(r)} \leftarrow \partial q/\partial x|_{x=x_i^{(r)}}\, \dot{x}_i^{(r)}$ ▷ *Jacobian–vector product*
10:     $\mathcal{L}_{\mathrm{geodesic}}^{(r)} \leftarrow \frac{1}{N_{\mathrm{image}}} \sum_{i=1}^{N_{\mathrm{image}}} \|\dot{q}_i^{(r)}\|^2$ ▷ *Geodesic loss*
11:   $\mathcal{L}_{\mathrm{geodesic}} \leftarrow \frac{1}{N_{\mathrm{rxn}}} \sum_{r=1}^{N_{\mathrm{rxn}}} \mathcal{L}_{\mathrm{geodesic}}^{(r)}$
12:   $\theta \leftarrow$ UPDATE$(\theta, \nabla_\theta \mathcal{L}_{\mathrm{geodesic}})$
13: **until** Convergence
14: **output** Optimized model parameters $\theta^*$

## S1.4 Hyperparameters

Model hyperparameters are listed in Table S1, and training hyperparameters for geodesic pre-training and energy-based training are provided in Table S2 and Table S3, respectively.

**Algorithm S2** Energy-based training (MEPIN-**L**)

**Require:** Reactant-product dataset $\mathcal{D}$, pre-trained parameters $\theta$

**repeat**

  **for** $r = 1, \cdots, N_{\text{rxn}}$ **do** ▷ *Reaction batch*

    Sample reactant and product pair $(x_{\text{R}}^{(r)}, x_{\text{P}}^{(r)}, a) \sim \mathcal{D}$

    $x_{\text{R}}^{(r)}, x_{\text{P}}^{(r)} \leftarrow \textsc{Augment}(x_{\text{R}}^{(r)}, x_{\text{P}}^{(r)})$

    **for** $i = 1, \cdots, N_{\text{image}}$ **do** ▷ *Image batch*

      Sample interpolation parameter $t_i \sim \mathcal{U}(0, 1)$

      $x_{\text{interp},i}^{(r)} \leftarrow (1 - t_i)x_{\text{R}}^{(r)} + t_i x_{\text{P}}^{(r)}$ ▷ *Initial interpolant (linear)*

      $x_i^{(r)} \leftarrow x_{\text{interp},i}^{(r)} + t_i(1 - t_i)\phi(x_{\text{R}}^{(r)}, x_{\text{P}}^{(r)}, x_{\text{interp},i}^{(r)}, a^{(r)}, t_i; \theta)$ ▷ *Predicted path image*

    $\mathcal{L}_{\text{flux}}^{(r)} \leftarrow \frac{1}{\beta} \log \left( \frac{1}{N_{\text{image}}} \sum_{i=1}^{N_{\text{image}}} \exp(\beta U(x_i^{(r)})) \|\dot{x}_i^{(r)}\| \right)$ ▷ *Flux loss*

    $\mathcal{L}_{\text{arc}}^{(r)} \leftarrow \frac{1}{N_{\text{image}}} \sum_{i=1}^{N_{\text{image}}} \langle \dot{x}_i^{(r)}, \ddot{x}_i^{(r)} \rangle^2$ ▷ *Arc length loss*

  $\mathcal{L}_{\text{energy}} \leftarrow \frac{1}{N_{\text{rxn}}} \sum_{r=1}^{N_{\text{rxn}}} \left( \mathcal{L}_{\text{flux}}^{(r)} + w_{\text{arc}} \mathcal{L}_{\text{arc}}^{(r)} \right)$

  $\theta \leftarrow \textsc{Update}(\theta, \nabla_\theta \mathcal{L}_{\text{energy}})$

**until** Convergence

**output** Optimized model parameters $\theta^*$

**Algorithm S3** Energy-based training (MEPIN-**G**)

**Require:** Reactant-product dataset $\mathcal{D}$, initial parameters $\theta$

**repeat**

  **for** $r = 1, \cdots, N_{\text{rxn}}$ **do** ▷ *Reaction batch*

    Sample reactant and product pair $(x_{\text{R}}^{(r)}, x_{\text{P}}^{(r)}, a) \sim \mathcal{D}$

    Get (cached) control points $\{x_{\text{geodesic},k}^{(r)}\}_{k=1}^{N_{\text{control}}}$ from geodesic interpolation

    **for** $i = 1, \cdots, N_{\text{image}}$ **do** ▷ *Image batch*

      Sample interpolation parameter $t_i \sim \mathcal{U}(0, 1)$

      $x_{\text{interp},i}^{(r)} \leftarrow f_{\text{spline}}(\{x_{\text{geodesic},k}^{(r)}\}, t_i)$ ▷ *Initial interpolant (geodesic)*

      $x_i^{(r)} \leftarrow x_{\text{interp},i}^{(r)} + t_i(1 - t_i)\phi(x_{\text{R}}^{(r)}, x_{\text{P}}^{(r)}, x_{\text{interp},i}, a^{(r)}, t_i; \theta)$ ▷ *Predicted path image*

    $\mathcal{L}_{\text{flux}}^{(r)} \leftarrow \frac{1}{\beta} \log \left( \frac{1}{N_{\text{image}}} \sum_{i=1}^{N_{\text{image}}} \exp(\beta U(x_i^{(r)})) \|\dot{x}_i^{(r)}\| \right)$ ▷ *Flux loss*

    $\mathcal{L}_{\text{arc}}^{(r)} \leftarrow \frac{1}{N_{\text{image}}} \sum_{i=1}^{N_{\text{image}}} \langle \dot{x}_i^{(r)}, \ddot{x}_i^{(r)} \rangle^2$ ▷ *Arc length loss*

  $\mathcal{L}_{\text{energy}} \leftarrow \frac{1}{N_{\text{rxn}}} \sum_{r=1}^{N_{\text{rxn}}} \left( \mathcal{L}_{\text{flux}}^{(r)} + w_{\text{arc}} \mathcal{L}_{\text{arc}}^{(r)} \right)$

  $\theta \leftarrow \textsc{Update}(\theta, \nabla_\theta \mathcal{L}_{\text{energy}})$

**until** Convergence

**output** Optimized model parameters $\theta^*$

Table S1: Model hyperparameters.

| Description | Transition1x | [3+2] Cyclo. |
|---|---|---|
| Number of feature dimensions | 64 | 32 |
| Number of radial basis functions | 20 | 20 |
| Number of message passing layers | 4 | 3 |
| Radius cutoff for edge construction $r_{\text{cut}}$ [Å] | 6.0 | 6.0 |
| Radius offset for radial basis function $r_{\text{shift}}$ [Å] | 0.5 | 0.5 |

Table S2: Geodesic pre-training (MEPIN-**L**) hyperparameters.

| Description | Transition1x | [3+2] Cyclo. |
|---|---|---|
| Number of reactions in batch $N_{\text{rxn}}$ | 3 | 3 |
| Number of images per reaction $N_{\text{image}}$ | 8 | 8 |
| Swap reactant and product randomly | True | False |
| Rotational augmentation angle scale $\sigma_{\text{angle}}$ [rad] | 0.05 | 0.05 |
| Learning rate | 0.0001 | 0.0001 |
| Internal coordinate short-range parameter $\bar{\alpha}$ | 1.7 | 1.7 |
| Internal coordinate long-range parameter $\bar{\beta}$ | 0.01 | 0.01 |
| Internal coordinate distance clamp [Å] | 0.1 | 0.1 |
| Geodesic loss clip value | 100 | 100 |
| Gradient clipping norm [a.u.] | 1 | 1 |

Table S3: Energy-based training (MEPIN-**L** and **G**) hyperparameters.

| Description | Transition1x | [3+2] Cyclo. |
|---|---|---|
| Number of reactions in batch $N_{\text{rxn}}$ | 4 | 4 |
| Number of images per reaction $N_{\text{image}}$ | 8 | 6 |
| Number of geodesic control points $N_{\text{control}}$ (**G**) | 11 | 11 |
| Swap reactant and product randomly | True (**L**) False (**G**) | False |
| Rotational augmentation angle scale $\sigma_{\text{angle}}$ [rad] | 0.05 (**L**) 0 (**G**) | 0.05 (**L**) 0 (**G**) |
| Learning rate | 0.0003 | 0.0003 |
| Flux loss inverse temperature $\beta$ [eV$^{-1}$] | 20 | 20 |
| Flux loss clip value [eV] | 50 | 50 |
| Arc length loss clip value [Å$^4$] | 500 | 500 |
| Arc length loss weight $w_{\text{arc}}$ [eV/Å$^4$] | 0.001 | 0.001 |
| Gradient clipping norm [a.u.] | 10 | 10 |

# S2 Dataset

## S2.1 Dataset Preparation

We randomly split the original Transition1x[S9] and [3+2] cycloaddition[S10] datasets into 90:10 train:test fractions. Validation sets were randomly sampled as 10% of each training split. All reactant and product complexes were re-optimized on the GFN1-xTB potential energy surface using xtb 6.5.1[S11]. Reactions were retained if the connectivity matrices of the optimized structures matched those of the original structures.

For test set reactions, transition state optimizations were performed on the GFN1-xTB surface using xtb 6.5.1 via the Scine xtb wrapper[S12]. Optimizations used the P-RFO algorithm[S13] with the Bofill Hessian update[S14], as implemented in Scine ReaDuct[S15]. If this failed to yield a saddle point with exactly one imaginary frequency, two fallback methods were attempted: the Dimer algorithm[S16,S17] and a double-ended B-spline-based optimization[S18], both also implemented in Scine ReaDuct.

Successful TS optimizations were followed by IRC calculations. The resulting endpoints were compared to the previously optimized reactant and product structures using Scine Molassembler[S19,S20]. The test set was filtered to include only IRC-verified reactions, retaining those for which both IRC endpoints matched the re-optimized structures within an RMSD cutoff of 0.25 Å.

## S2.2 Comparison with the Original Dataset

In addition to additional test set filtering to ensure the reference IRC path connects the identified TS with the reactant and product (with an endpoint RMSD below 0.25 Å for both), the dataset here differs from the original one in two main ways: (1) the level of theory is reduced from DFT to GFN1-xTB, and (2) for the Transition1x set, TS structures are now IRC-confirmed rather than obtained via CI-NEB[S9]. To assess whether these changes affect reaction characteristics, we compare energetics and geometries for the test split of

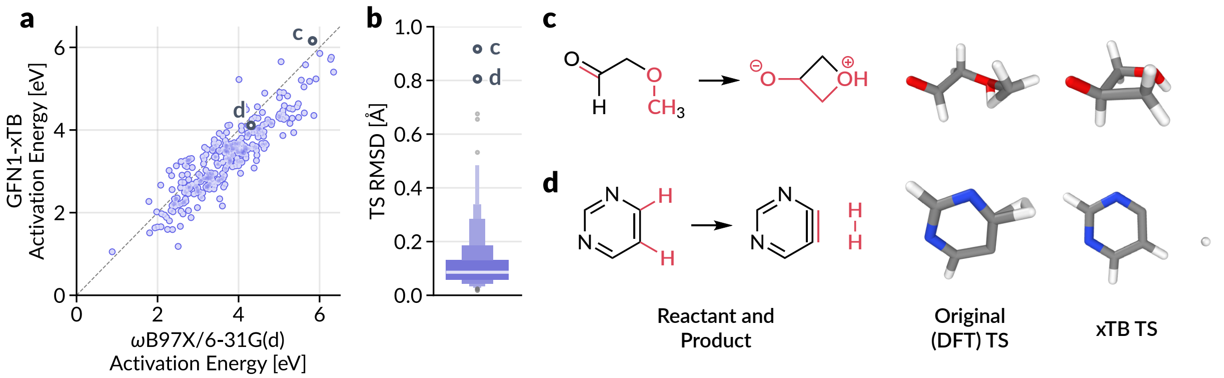


Figure S1: Comparison between the original Transition1x dataset[S9] and the updated GFN1-xTB-based dataset. (a) Activation energies using reactant and TS structures from the original ($\omega$B97X/6-31G(d)) and current (GFN1-xTB) datasets. (b) RMSD between TS geometries in the two datasets, with most values low except for a few outliers. (c, d) Reactions and TS structures from the original and current work for two annotated outlier cases.

Transition1x dataset used here.

As shown in Fig. S1a, activation energies from the original ($\omega$B97X/6-31G(d)) and current (GFN1-xTB) datasets align closely with $y = x$ line. Similarly, Fig. S1b shows low RMSD values between TS structures across datasets, with a few outliers. These outliers involve charge-separated products with competing pathways (Fig. S1c) or evolution of molecular hydrogen with distorted original TS geometry (Fig. S1d). Overall, the results indicate that, except for few exceptions, the GFN1-xTB-based pipeline in this work maintains consistent reaction energetics and TS geometries.

# S3 Additional Results

## S3.1 Saddle-Point Optimization

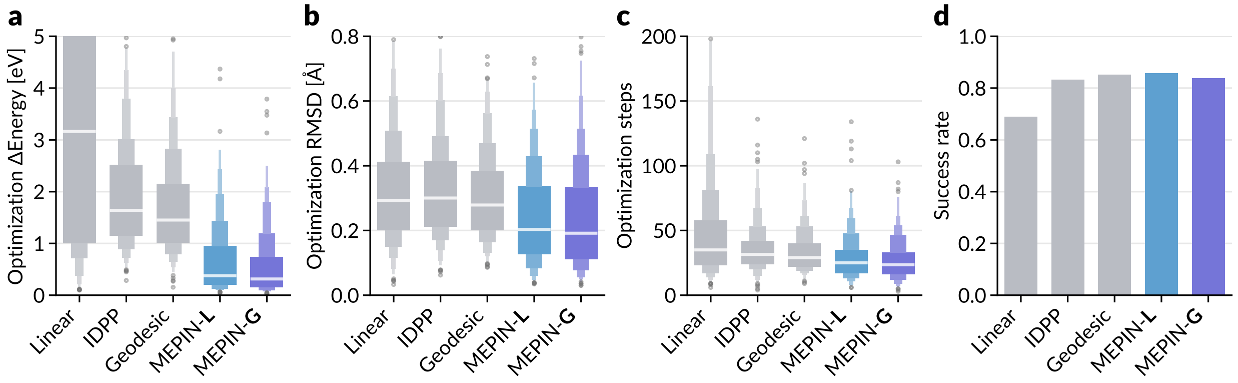


Figure S2: Saddle-point optimization results for the Transition1x test set using initial TS geometries from interpolations and reaction path models. (a) Energy change during optimization. (b) RMSD between initial and optimized geometries. (c) Number of steps required for convergence. (d) Optimization success rate, defined as RMSD to reference TS $< 0.2$ Å.

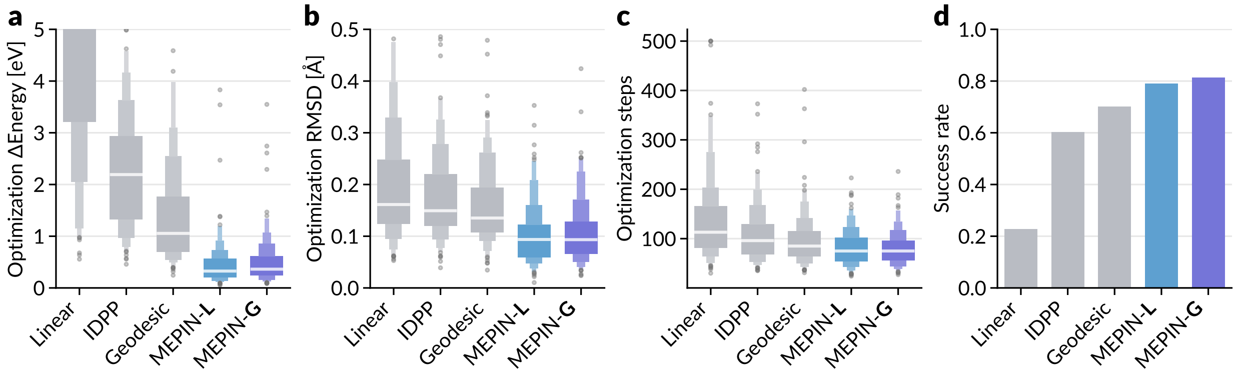


Figure S3: Saddle-point optimization results for the [3+2] cycloaddition test set using initial TS geometries from interpolations and reaction path models. (a) Energy change during optimization. (b) RMSD between initial and optimized geometries. (c) Number of steps required for convergence. (d) Optimization success rate, defined as RMSD to reference TS $< 0.2$ Å.

In addition to the IRC-based path comparisons in the main text, we performed saddle-point optimizations of predicted TSs from each interpolation method and reaction path model. Results for the Transition1x and [3+2] cycloaddition test sets are shown in Figs. S2 and S3, respectively. Optimizations were performed with the Sella optimizer[S21] until the

maximum residual force component was less than 0.05 eV/Å. The learned models place the highest-energy image closer to the true saddle point, both energetically (panels a) and geometrically (panels b), reducing required optimization steps (panels c). For [3+2] cycloadditions, optimized saddle points better match reference TS structures, particularly in cases where geometric interpolations struggle with large reactants. These results demonstrate that reaction path models provide more accurate initial guesses and improve TS refinement efficiency.

## S3.2 Inference Example: Energy vs. Geometry

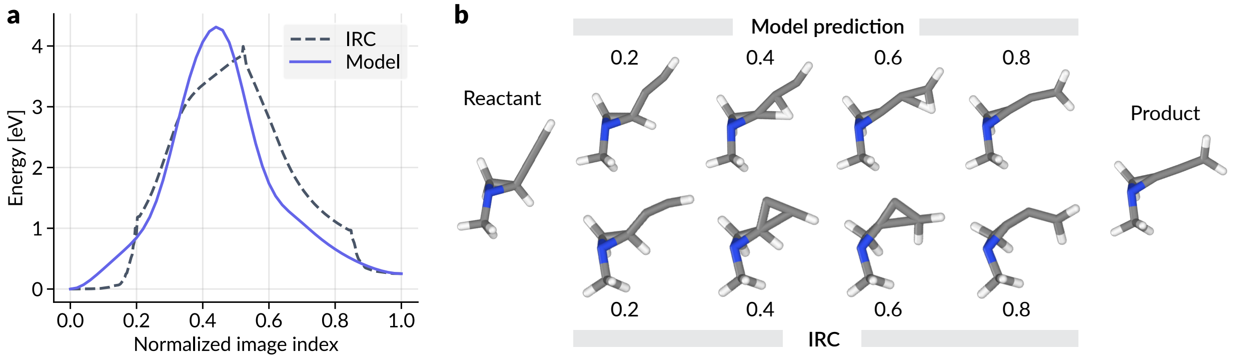


Figure S4: Reaction profile for the 1,3-hydrogen shift from alkyne to allene in the Transition1x test set. (a) Energy profile along the reaction path from IRC and MEPIN-**L** predictions, plotted against the normalized image index (0 to 1). Note that the parametrization of the $x$-axis is relatively arbitrary, especially for the IRC, where the tails may appear elongated due to smaller gradients and asymmetric convergence rates between the forward and reverse directions. The position of the TS along the $x$-axis does not necessarily correspond to its actual structural distance from the reactants or products. (b) Evolution of the 3D geometries from IRC and model predictions, labeled with normalized image indices. While both paths exhibit similar energetics, they have relatively a large geometric difference, with a moderate TS energy difference of 0.32 eV and a large RMSD of 0.77 Å.

Fig. S4 shows an inference example using the trained MEPIN-**L** for a reaction from the Transition1x test set. In Fig. S4a, the energy profile is plotted against a normalized image index from 0 to 1 (note that the $x$-axis parametrization is arbitrary with respect to geometric progress, as noted in the caption), showing good energy agreement with a maximum deviation of 0.32 eV. However, the model-predicted path differs significantly from the IRC in geometry,

with a TS RMSD of 0.77 Å. Despite this, the predicted path remains physically meaningful, highlighting that geometric agreement with the reference path is not a sufficient metric for assessing the reaction model performance—particularly when the model is trained solely with an energy-based objective.

## S3.3 Computational Cost

Geodesic pre-training was performed on a single NVIDIA A100 (40GB) GPU and took approximately 6 hours to converge. Energy-based training was conducted on a compute node with four NVIDIA A100 (40GB) GPUs and required 70–90 hours until convergence. The difference in training time is primarily due to GFN1-xTB energy evaluations using the dxtb package[S6] on GPU. Although GPU was used here for implementation convenience, these evaluations can be offloaded to CPU resources, which may accelerate training given sufficient CPU resource availability.

Table S4: Average runtime (in ms) for each interpolation method and reaction path model.

| Dataset | Num. images | Linear | IDPP | Geodesic | MEPIN-**L** | | MEPIN-**G**† | |
|---|---|---|---|---|---|---|---|---|
| | | | | | GPU | CPU | GPU | CPU |
| Transition1x | 11 | 0.09 | 92 | 510 | 10.5 | 106 | 10.1 | 112 |
| | 21 | 0.09 | 200 | 1080 | 11.1 | 150 | 11.0 | 161 |
| | 51 | 0.11 | 477 | 4000 | 19.2 | 278 | 19.0 | 310 |
| [3+2] Cycloaddition | 11 | 0.11 | 119 | 4420 | 11.6 | 322 | 12.9 | 269 |
| | 21 | 0.13 | 259 | 7650 | 14.0 | 545 | 17.0 | 517 |
| | 51 | 0.17 | 633 | 21 000 | 21.7 | 1550 | 24.2 | 1480 |

† MEPIN-**G** inference time is reported excluding the computation time for the (cached) geodesic control points. Including geodesic interpolation with 11 images, the full inference time increases by 510 ms for Transition1x and 4420 ms for [3+2] cycloaddition.

The average runtime for each interpolation method and reaction path model is reported in Table S4. Runtimes are measured using a single NVIDIA A100 (40GB) GPU and 20 cores of an Intel Xeon Gold 6248 CPU. Even on CPU, model inference is comparable to or faster than geometric interpolation methods that require optimization (IDPP and geodesic).

# References

(S1) Schütt, K.; Unke, O.; Gastegger, M. Equivariant message passing for the prediction of tensorial properties and molecular spectra. Proceedings of the 38th International Conference on Machine Learning. 2021; pp 9377–9388.

(S2) Nam, J.; Liu, S.; Winter, G.; Jun, K.; Yang, S.; Gómez-Bombarelli, R. Flow Matching for Accelerated Simulation of Atomic Transport in Materials. 2025; https://arxiv.org/abs/2410.01464.

(S3) Schreiner, M.; Winther, O.; Olsson, S. Implicit Transfer Operator Learning: Multiple Time-Resolution Models for Molecular Dynamics. Advances in Neural Information Processing Systems. 2023; pp 36449–36462.

(S4) Zhu, X.; Thompson, K. C.; Martínez, T. J. Geodesic interpolation for reaction pathways. *J. Chem. Phys.* **2019**, *150*.

(S5) Bartels, R. H.; Beatty, J. C.; Barsky, B. A. *An introduction to splines for use in computer graphics and geometric modeling*; Morgan Kaufmann, 1995.

(S6) Friede, M.; Hölzer, C.; Ehlert, S.; Grimme, S. dxtb—An efficient and fully differentiable framework for extended tight-binding. *J. Chem. Phys.* **2024**, *161*.

(S7) Grimme, S.; Bannwarth, C.; Shushkov, P. A robust and accurate tight-binding quantum chemical method for structures, vibrational frequencies, and noncovalent interactions of large molecular systems parametrized for all spd-block elements (Z=1–86). *J. Chem. Theory Comput.* **2017**, *13*, 1989–2009.

(S8) Kingma, D. P.; Ba, J. Adam: A Method for Stochastic Optimization. 2014; https://arxiv.org/abs/1412.6980.

(S9) Schreiner, M.; Bhowmik, A.; Vegge, T.; Busk, J.; Winther, O. Transition1x-a dataset

for building generalizable reactive machine learning potentials. *Sci. Data* **2022**, *9*, 779.

(S10) Stuyver, T.; Jorner, K.; Coley, C. W. Reaction profiles for quantum chemistry-computed [3+2] cycloaddition reactions. *Sci. Data* **2023**, *10*, 66.

(S11) Bannwarth, C.; Caldeweyher, E.; Ehlert, S.; Hansen, A.; Pracht, P.; Seibert, J.; Spicher, S.; Grimme, S. Extended tight-binding quantum chemistry methods. *Wiley Interdiscip. Rev.: Comput. Mol. Sci.* **2021**, *11*, e1493.

(S12) Bensberg, M.; Csizi, K.-S.; Grimmel, S. A.; Sobez, J.-G.; Steiner, M.; Türtscher, P. L.; Unsleber, J. P.; Reiher, M. qcscine/xtb_wrapper: Release 3.0.1. 2024; https://doi.org/10.5281/zenodo.13372943.

(S13) Banerjee, A.; Adams, N.; Simons, J.; Shepard, R. Search for stationary points on surfaces. *J. Phys. Chem.* **1985**, *89*, 52–57.

(S14) Bofill, J. M. Updated Hessian matrix and the restricted step method for locating transition structures. *J. Comp. Chem.* **1994**, *15*, 1–11.

(S15) Bensberg, M.; Brunken, C.; Csizi, K.-S.; Grimmel, S. A.; Gugler, S.; Sobez, J.-G.; Steiner, M.; Türtscher, P. L.; Unsleber, J. P.; Vaucher, A.; Weymuth, T.; Reiher, M. qcscine/readuct: Release 6.0.0. 2024; https://doi.org/10.5281/zenodo.13372944.

(S16) Kästner, J.; Sherwood, P. Superlinearly converging dimer method for transition state search. *J. Chem. Phys.* **2008**, *128*.

(S17) Shang, C.; Liu, Z.-P. Constrained Broyden minimization combined with the dimer method for locating transition state of complex reactions. *J. Chem. Theory Comput.* **2010**, *6*, 1136–1144.

(S18) Vaucher, A. C.; Reiher, M. Minimum Energy Paths and Transition States by Curve Optimization. *J. Chem. Theory Comput.* **2018**, *14*, 3091–3099.

(S19) Sobez, J.-G.; Reiher, M. Molassembler: Molecular Graph Construction, Modification, and Conformer Generation for Inorganic and Organic Molecules. *J. Chem. Inf. Model.* **2020**, *60*, 3884–3900.

(S20) Bensberg, M.; Grimmel, S.; Sobez, J.-G.; Steiner, M.; Unsleber, J. P.; Reiher, M. qcscine/molassembler: Release 3.0.0. 2024; https://doi.org/10.5281/zenodo.13372940.

(S21) Hermes, E. D.; Sargsyan, K.; Najm, H. N.; Zádor, J. Sella, an open-source automation-friendly molecular saddle point optimizer. *J. Chem. Theory Comput.* **2022**, *18*, 6974–6988.
